# Supplementary material for: Terrain RL Simulator
Source: arXiv:1804.06424 source file (2018-04-17)
Supplement: Supplementary file 1 [file paper_appendix.tex]

\addcontentsline{toc}{chapter}{Appendix}
\section{Appendix}
\label{sec:Appendix}
